# Supplementary material for: MODNet -- accurate and interpretable property predictions for limited materials datasets by feature selection and joint-learning
Source: arXiv:2004.14766 ancillary file (2021-07-07)
Supplement: Supplementary file 1 [file suppl.pdf]

## Supplemental Material

### Machine learning materials properties for small datasets

Pierre-Paul De Breuck, Geoffroy Hautier and Gian-Marco Rignanese

*Université catholique de Louvain (UCLouvain),  
Institute of Condensed Matter and Nanosciences (IMCN),  
Chemin des Étoiles 8, B-1348 Louvain-la-Neuve, Belgium*

## I. SUPPLEMENTARY METHODS AND DISCUSSION

### A. Datasets

The different models used in this work were trained on four different properties: formation energy, band gap, refractive index and vibrational thermodynamics. We briefly present these latter two datasets as they are new to the machine learning field. Petretto *et al.* [1] computed the vibrational properties for 1,245 inorganic compounds, in the harmonic approximation based on Density Functional Perturbation Theory (DFPT). In particular, this dataset contains the following thermodynamic properties: vibrational entropy, Helmholtz free energy, internal energy and heat capacity from 5 to 800 K in steps of 5 K. Figure S1 graphically represents these four properties from 5 to 800 K for all materials contained in the dataset in meV/atom or meV/K/atom. A wide variety of values is reached, with different Debye temperatures as can be seen from the specific heat. This is important to notice as it indicates that there is no significant bias, giving us confidence for generalizing on unseen data.

The refractive index for 4028 compounds were computed by Naccarato *et al.* (see Ref. [2]) relying on Density Functional Theory (DFT) and high-throughput methods. Typical values encountered in the dataset ranges from 1 to 6, with 60% below 2.

Figures S2, S3 and S4 contain various histograms representing the data distribution for both properties. Various crystalline compounds are present ranging from simple mono-elemental compounds to complex semiconductors. The thermodynamic data (resp. refractive index) cover the 7 (resp. 7) symmetry groups, 84 (resp. 165) space groups and 64 (resp. 86) elements. Most compounds are ternary alloys and there are no (resp. almost no) materials with more than 5 different elements. The mean atomic mass has a large range, confirming the variety of elements present in these two datasets. Note that the refractive index dataset is biased towards oxides, with 27 % of all materials containing oxygen atoms.

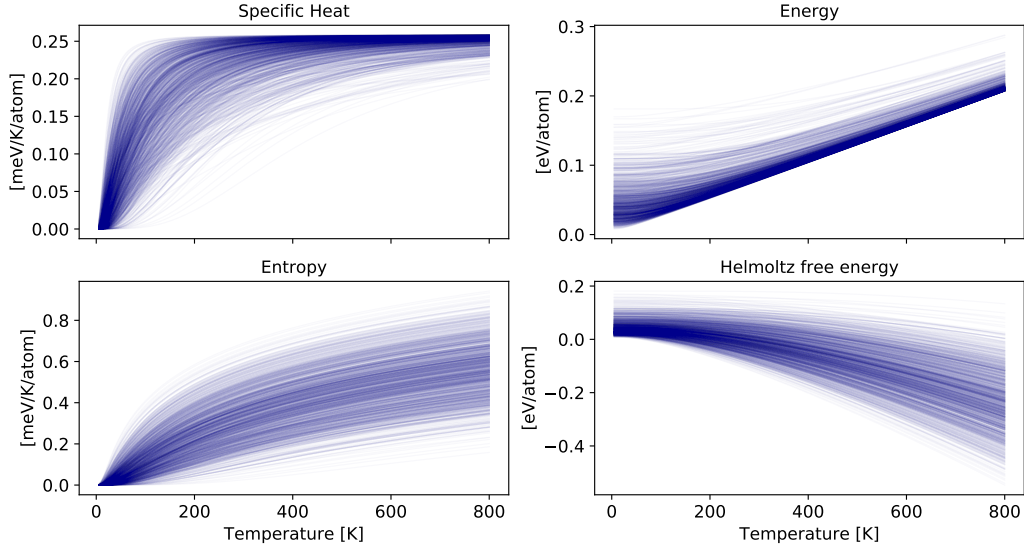

Figure S1. Visual representation of values encountered in the vibrational thermodynamic dataset (from Ref. [1]). Four vibrational properties from 5 to 800 K for 1245 materials are present. A wide range of values are reached, with clear differences in Debye temperatures.

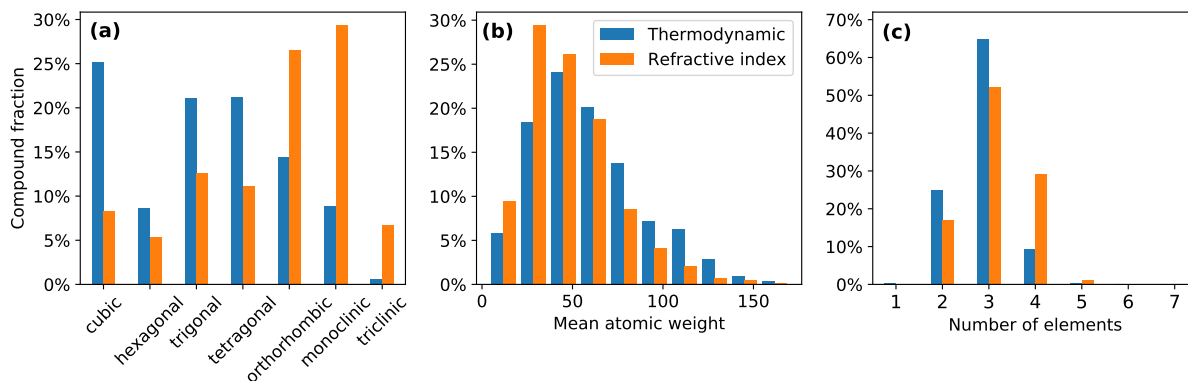

Figure S2. Relative distribution of (a) the crystal system, (b) mean atomic mass and (c) number of elements for both the thermodynamic and refractive index datasets.

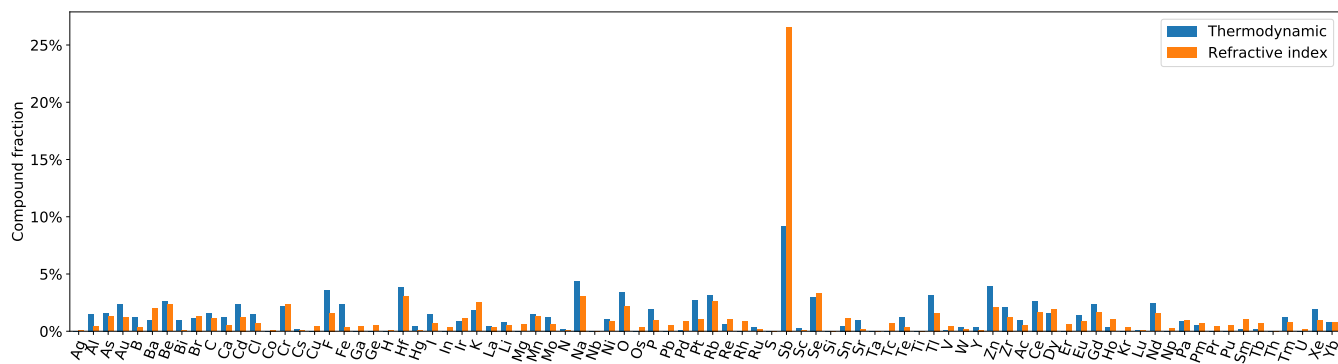

Figure S3. Relative amount of samples containing a particular element for both the thermodynamic and refractive index datasets. In total, they cover 64 and 86 elements respectively.

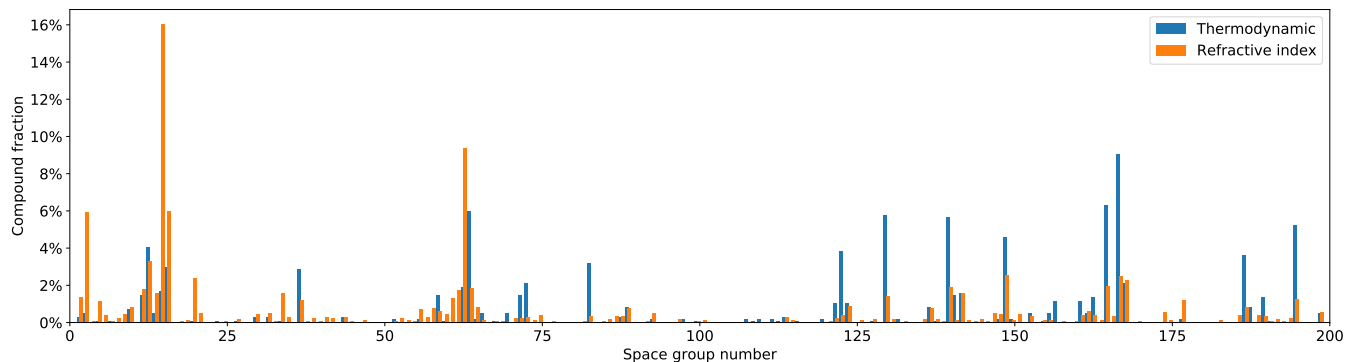

Figure S4. Space group distribution for both the thermodynamic and refractive index datasets. In total they cover 84 and 165 spacegroups respectively.

## B. Identifying compound-property relations with feature selection

The presented feature selection algorithm enables one to find an optimal subset of descriptors. As they are chosen according to their relation (i.e. mutual information), important factors contributing to the target property can be found. Figure S5 shows a bivariate visualization for the vibrational entropy, formation energy, band gap and refractive index as a function of the two first selected features. Thanks to the redundancy criterion, both features are

complementary to predict the target. A detailed description of these features can be found at the end of this section.

Concerning the vibrational entropy, a strong correlation is seen with the first feature, namely *AGNIFingerprint*, which gives a measure of the inverse bond length. In other words, increasing the average bond length increases the vibrational entropy. Similarly having a larger range of p-valence electrons (which is linked to ionicity) increases the vibrational entropy. Concerning the refractive index, two import factors are identified: the band gap and the density of the material. The band gap, although not explicitly given but instead approximated by the bandgap of the constituent elements, is known to be an important variable. Typically there is an inverse relation between the band gap energy and the refractive index, see Ref. [2]. Finding materials combining a high value for both properties remains a tedious task, and could therefore certainly benefit from Machine Learning.

Overall, it is seen how common intuitive patterns for the physicist are indeed retrieved by the machine. Therefore, we are convinced that this strategy can be used to analyze and find underlying factors for all types of properties.

- **AGNIFingerprint:** This feature represents the local environment of an atom by computing the integral of the product of the radial distribution function (RDF) with a Gaussian window function. It was originally proposed by Botu *et al.* to fit empirical energy potentials [3]. It is defined as:

$$G_i(\eta) = \int R_i(r) e^{-\left(\frac{r_{ij}}{\eta}\right)^2} dr \quad (\text{S1})$$

where  $i$  is the considered site,  $R(r)$  the RDF,  $r_{ij}$  the distance between site  $i$  and neighbor  $j$  and  $\eta$  giving the width of the Gaussian window. In practice, this integral is discretized and a cut-off function is used, see the original work for more information [3].

When computed for a compound, the mean *AGNIFingerprint* over all sites is taken.

- **p-valence range:** Range of p-electrons, i.e. the number of p-electrons is first computed for each element in the compound, and then the difference between the highest and lowest number is taken.
- **Maximum GS bandgap** Highest bandgap among the ground state (GS) constituent elemental compounds. In other words, for each element in the composition, the corresponding most stable single-elemental structure is taken with a corresponding band gap. Then the maximum over these different elemental bandgaps is taken.
- **Density:** Mass per unit volume of the compound.
- **Minimum  $\Delta\chi$ :** Here  $\Delta\chi$  represents the difference in electronegativity between a given cation and the mean electronegativity of all anions in the compound. This is first computed for each cation. Then the minimum is taken over all cations.
- **Generalized RDF:** This featurizer generalizes the RDF by using non-rectangular bins (Gaussian binning is used here), see Ref. [4]. It is therefore very similar to the previously explained *AGNIFingerprint*. Here the integral of the RDF with a Gaussian of mean 4.0 Å and width 1.0 Å is taken.
- **HOMO:** The highest occupied molecular orbital (HOMO) is estimated from the atomic orbital energies of the composition (see Ref. [5]).
- **Maximum Packing Efficiency:** This feature (see Ref. [6]) represents the packing efficiency of the crystal by measuring the volume fraction of occupied atoms. The algorithm first determines the largest radius for each atom, which equals the distance from the center of the atom to the closest Voronoi face. Then, the packing efficiency is computed as the following volume ratio:

$$\frac{1}{V_{cell}} \sum_i \frac{4}{3} \pi r_i^3 \quad (\text{S2})$$

where  $V_{cell}$  is the volume of the unit cell and  $r_i$  the largest radius (as defined before) of each atom  $i$  in the unit cell.

Note that, exceptionally, some features are unable to be computed for a few compounds, due to missing information needed by the underlying routines. When this happens, the corresponding value is set to -1, which explains negative values for non-negative properties in Fig. S5.

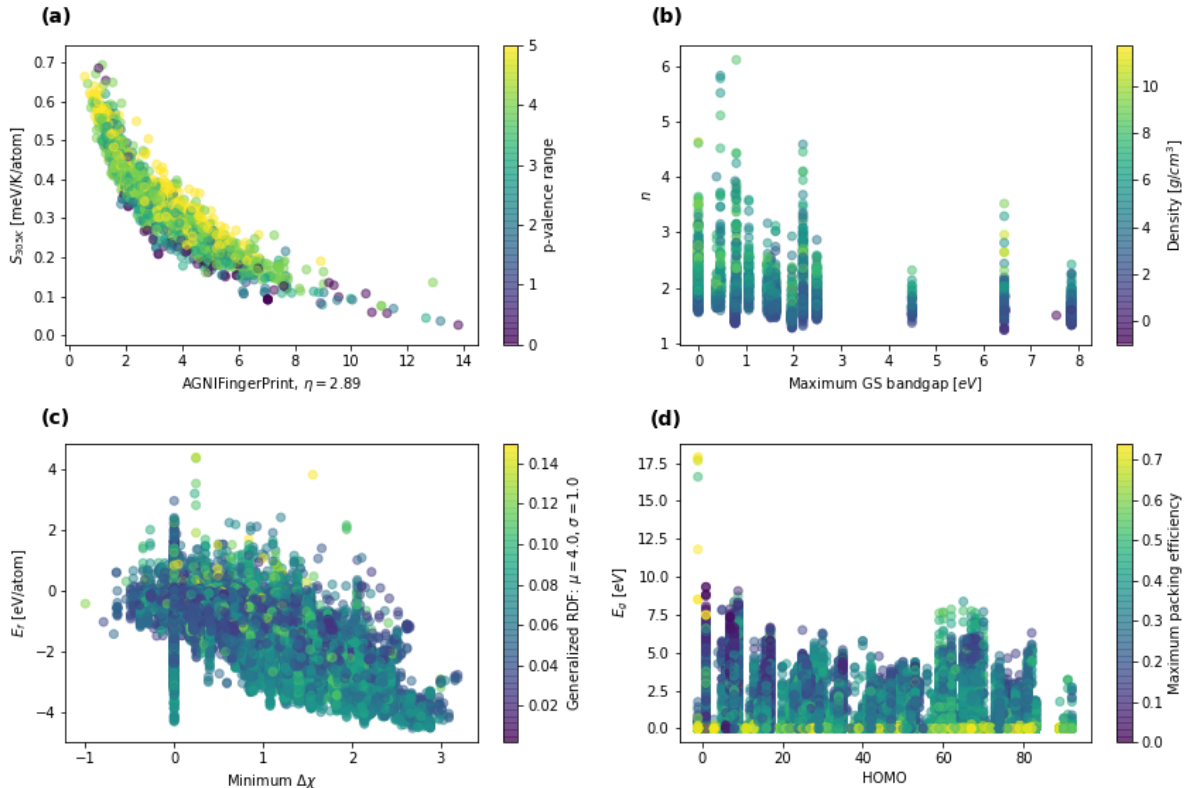

Figure S5. Bivariate representation of the two most important features for four different properties: (a) vibrational entropy at 305 K, (b) refractive index, (c) formation energy and (d) band gap energy. Both features are complementary to narrow down the target output, although certainly not sufficient for an accurate estimation.

### C. Model testing procedure

For assessing the performance of a model, we follow the standard procedure which consists in splitting the dataset in mutually exclusive training, validation and test sets. Validation is used in order to optimize the hyperparameters, while the test set is used for obtaining an unbiased generalization performance for the best hyperparameters. The Mean Absolute Error (MAE) is systematically used as performance criterion. Moreover, all datasets that are considered as small (i.e. all properties except the full formation and band gap energy sets covering 60 000 materials) use a 10-fold validation scheme. Table S1 summarizes training, validation and test set sizes for each property used in this work.

Concerning the hyperparameters, for neural networks they consist in the number of layers, number of neurons per layer, learning rate, batch size, activation function and loss function. The MODNet has an additional hyperparameter consisting in the number of optimal input features. The MEGNet has also an additional hyperparameter consisting in the number of MEGNet-blocks. Finally, when using the Random Forest the number of trees is taken as the only hyperparameter. As an in depth-example, the next section discusses how the hyperparameters were chosen for the MODNet when trained on multiple vibrational thermodynamic quantities.

Table S1. Training, validation and test sizes used for training the models on the different datasets, see Table I of the main paper. All properties (except the complete formation and band gap energy datasets) use a 10-fold cross validation scheme. Validation sizes always correspond to 1/10th of the total train-validation set.

| Property   | Training size | Validation size | Test size |
|------------|---------------|-----------------|-----------|
| $E_f$      | 504           | 56              | 4990      |
|            | 60 000        | 6 667           | 1 822     |
| $E_g$      | 504           | 56              | 4990      |
|            | 60 000        | 6 667           | 1 822     |
| $E_g^{nz}$ | 504           | 56              | 4990      |
|            | 36 720        | 4 080           | 4 628     |
| $n$        | 3 240         | 360             | 425       |
| $S_{305K}$ | 990           | 110             | 125       |

#### D. Hyperparameter optimization of MODNet when learning on multiple properties

Hyperparameter optimization is done following a 10-fold validation scheme on the previously presented dataset. The network is trained on 90% of the data, then validated on the remaining 10% by computing the MAE of each property (4 thermodynamic quantities, each at 20 temperatures). This is repeated ten times, and the mean over the ten folds is taken.

It is important to note that the network is optimized on all targets together. Therefore, different MAEs corresponding to different properties are combined to form the following criteria:

- **WMAE**: A Weighted summed MAE of the different properties such that the property-temperature curves are in the same range:

$$\text{WSMAE} = \sum_{p \in (S, C_v, H, U)} w_p \text{MAE}_p, \quad (w_S, w_{C_v}, w_H, w_U) = (0.3, 1, 0.004, 0.001) \quad (\text{S3})$$

- **MAX WSMAE**: The WSMAE, but only taking the 5% worst predicted samples.
- **MAPE**: A mean absolute percentage error over all properties.

First, the learning rate of MODNet was optimized to 0.01 from the set  $\{0.1, 0.1, 0.005, 0.001\}$ , by fixing all other hyperparameters on arbitrarily chosen values.

We then optimize the global loss function, by studying the effect of the following hyperparameters: input scaling, output scaling, loss function and loss weights. These two latter parameters are very important as the peculiarity of our network consists in optimizing the predictions of *multiple* targets. Therefore, each target should have an equal contribution in the loss functions. For example, the vibrational energy and enthalpy are typically 3 orders of magnitude larger than the vibrational entropy and specific heat, which causes an imbalance in the summation of the loss function. Different solutions exist, such as scaling the targets or weighting targets in the loss function.

Table S3 presents the MAE (over 10 folds) for various combinations of previous loss-parameters. For scaling, a min-max or standard scaling were tested. For the loss function, a Mean Square Error (MSE) or MAE were compared. Furthermore, weighting the 4 different properties such that the average property-temperature curves are in the same range was also compared against scaling. From the results (see Table S3), it was chosen to use a min-max scaling of the input variables, a MSE loss function and weighting of the different properties instead of scaling.

Once the learning rate, scaling, loss function and weighting are fixed, the number of layers as well as the number of neurons can be optimized. We choose two layers per block (except for the last one), with 256, 128, 64 and 8 neurons in the successive blocks, see Fig. S6. Adding (or removing) a layer, as well as doubling or halving the number of neurons does not improve accuracy as can be seen in Fig. S7. From the same figure, the batch size was fixed to 256. Other architectures that were tested are listed in Table S4 with the corresponding performance criteria. Finally, the number of features were optimized, see next section.

The final architecture is depicted in Fig. S6. A rectified linear unit function (ReLU) is used as activation for each layer. Learning is performed using an Adam optimizer ( $\beta_1 = 0.9$ ,  $\beta_2 = 0.999$ ,  $decay = 0$ ) on 600 epochs.

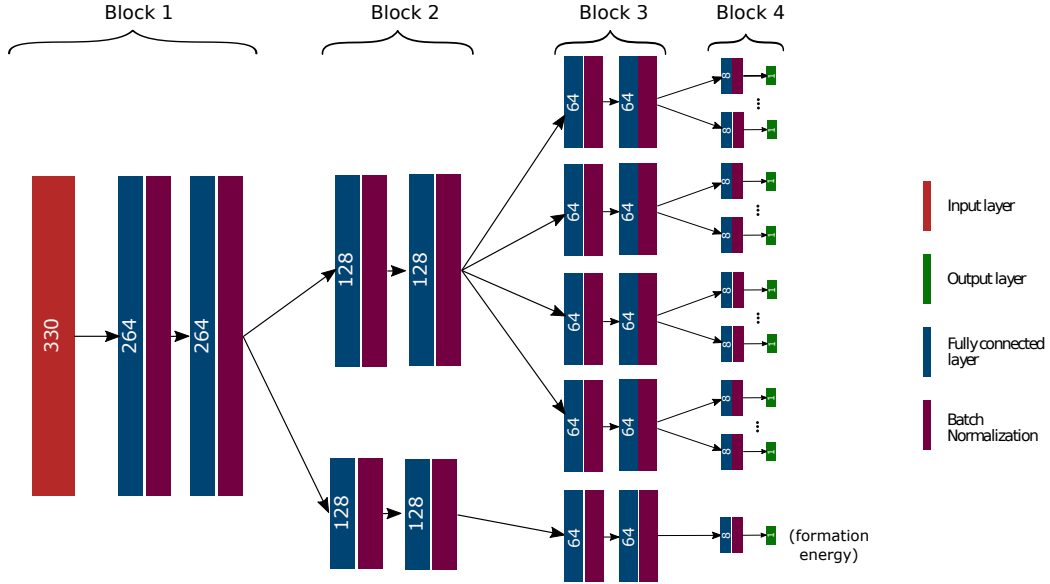

Figure S6. Architecture of the MODNet (composed of 4 blocks) when learning on the vibrational properties. The formation energy is added by adding a second order block to the first block.

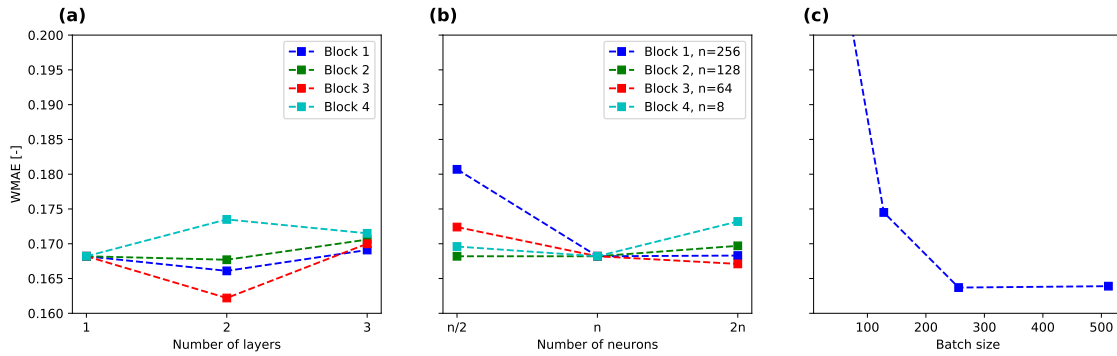

Figure S7. Optimization of the MODNet architecture. The effect of adding or removing layers (a) at each block is shown as well as reducing or increasing the number of neurons (b). The effect of changing the batch size is also shown (c). When one hyperparameter is changed, others are kept fixed at respectively 256, 128, 64 and 8 neurons (and 1 layer) per block.

Table S2. Architecture and hyperparameters of the MODNet for each property of Table I. Architecture is given in number of neurons per layer separated by a comma.

| Property | Training size | Architecture             | Activation | Loss | Batch size | Learning rate | # optimal features |
|----------|---------------|--------------------------|------------|------|------------|---------------|--------------------|
| $E_f$    | 504           | 256, 128                 | ReLU       | MAE  | 64         | 0.001         | 1000               |
|          | 60,000        | 1024, 256, 128           | ELU        | MAE  | 64         | 0.001         | 2000               |
| $E_g$    | 504           | 256, 128, 64, 64, 32, 32 | ELU        | MAE  | 64         | 0.001         | 1000               |
|          | 60,000        | 256, 128                 | ELU        | MAE  | 64         | 0.001         | 1000               |
| $n$      | 36,720        | 128, 64, 32              | ELU        | MAE  | 64         | 0.001         | 1000               |

Table S3. Scaling and loss optimization of MODNet when learning on the four vibrational properties and formation energy. The validation error (three custom defined criteria, see text, and  $S_{305K}$ ) is reported for each set of hyperparameters.

| Input scale | Output scale | Loss function | Loss weights <sup>a</sup> | WMAE   | MAX WMAE | MAPE   | $S_{305K}$ [meV/K/atom] |
|-------------|--------------|---------------|---------------------------|--------|----------|--------|-------------------------|
| min-max     | No           | MSE           | Yes, squared              | 0.167  | 0.435    | 0.0653 | 0.00860                 |
| Standard    | No           | MSE           | Yes, squared              | 0.185  | 0.482    | 0.0760 | 0.00959                 |
| No          | No           | MSE           | Yes, squared              | 0.416  | 1.220    | 0.158  | 0.0207                  |
| min-max     | No           | MAE           | Yes                       | 0.166  | 0.447    | 0.0683 | 0.00881                 |
| min-max     | min-max      | MAE           | No                        | 0.172  | 0.454    | 0.0700 | 0.00894                 |
| min-max     | min-max      | MAE           | No                        | 0.164  | 0.441    | 0.0680 | 0.00890                 |
| min-max     | min-max      | MSE           | No                        | 0.259  | 0.630    | 0.109  | 0.01253                 |
| min-max     | min-max      | MSE           | No                        | 0.1677 | 0.440    | 0.0666 | 0.00894                 |

Table S4. Supplementary architectures for optimization of MODNet when learning on the four vibrational properties and formation energy. The validation error (three custom defined criteria, see text, and  $S_{305K}$ ) is reported for each set of hyperparameters.

| Block 1      | Block 2  | Block 3  | Block 4 | WMAE   | WMAE MAX | MAPE   | $S_{305K}$ [meV/K/atom] |
|--------------|----------|----------|---------|--------|----------|--------|-------------------------|
| 256,256      | 128,128  | 64,64    | 8       | 0.166  | 0.434    | 0.0666 | 0.00873                 |
| 256,256      | 128,128  | 64,64    | 8,8     | 0.169  | 0.441    | 0.0679 | 0.00881                 |
| 128,128,128  | 64,64,64 | 32,32,32 | 8,8     | 0.182  | 0.468    | 0.0730 | 0.00945                 |
| 512          | 512      | 128      | 64      | 0.1646 | 0.429    | 0.0668 | 0.00866                 |
| 256, 128, 32 | 32, 32   | 32, 64   | 16      | 0.174  | 0.455    | 0.0712 | 0.00892                 |
| 512          | 128      | 64       | 8, 8, 8 | 0.1698 | 0.441    | 0.0688 | 0.00876                 |
| 512          | 128      | 64       | 4, 4, 4 | 0.1651 | 0.433    | 0.0658 | 0.00840                 |
| 512          | 128      | 16       | 3, 3, 3 | 0.1702 | 0.440    | 0.0686 | 0.00863                 |

### E. Optimal number of features for m-MODNet

The effect of the number of optimal features is assessed here. This is done by computing the MAE for  $S_{305K}$  of m-MODNet as a function of the number of relevant features. As one can observe in Fig. S8, the MAE is monotonically decreasing until  $\sim 330$  features, which shows that newly added features are indeed relevant to the prediction, followed by a gentle increase in MAE. One can thus safely ignore the remaining features. Note that the observed increase after the minimum is quite weak, and taking all computed features would not be dramatic. From our knowledge, this is because 2000 features is still small for a network such as the m-MODNet which drastically limits overfitting by its joint-nature. In contrast, the single target MODNet benefits much more from feature selection as was stated in the main paper. One could go beyond by computing even more features. For example, we recommend computing multiple functions ( $\frac{1}{x}, x^2, \log(x), e^x, \dots$ ), called feature engineering (see Ref. [7] for an empirical analysis), which would certainly improve predictions. Nevertheless, reducing the number of features is still beneficial in our case, as it slightly reduces the validation error, reduces computation time and moreover enables to identify (and understand) important features.

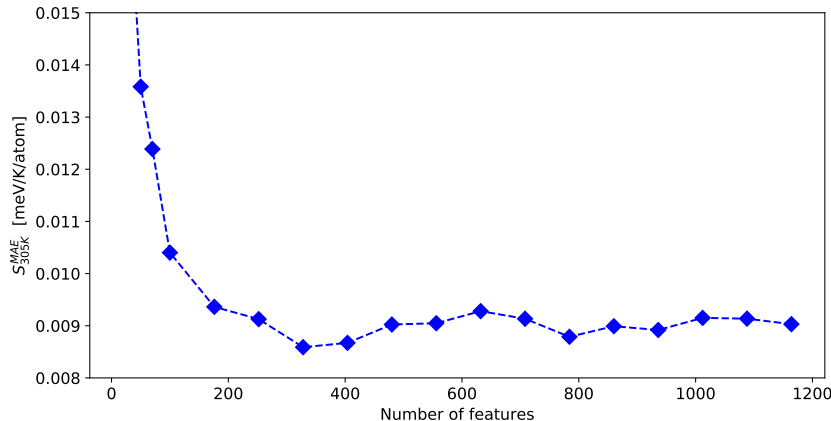

Figure S8. MAE of  $S_{305K}$  as a function of the number of features selected by our feature selection algorithm for m-MODNet.

## F. Practical considerations of SISSO

The screening and sparsifying operator (SISSO) model has been fitted on various properties in this work for comparison purposes. Some important practical aspects are detailed in this section.

The SISSO framework typically starts from a few tens of features, iteratively applies operators on them in order to generate an enormous amount of combined features before proceeding to the SISSO screening itself. In our work, we automatically generate thousands of features for each material. Using all of them as starting point in the SISSO-approach is in fact unfeasible as the amount of secondary and ternary features grow too quickly. Therefore, one should first select the most appropriate primary features before running the SISSO framework.

We chose to proceed as follow. A first SISSO is executed without any operators (i.e. rung set to 0), and with a SIS-subspace of 3 features. The 50-dimensional model is then used to select the corresponding 50 most significant features. Then a second SISSO is executed on these 50 features with a rung of 2 and SIS-space of 20 features. Then the best model equal or below 5D is chosen before being evaluated on the hold-out test set. In other words we use a double SISSO, with the first one used to do feature selection.

## G. Comparison with other feature selection methods

The feature selection algorithm presented in this work is based on the Normalized Mutual Information (NMI). Other popular choices exist and we choose to compare our algorithm with five other algorithms as a substitute:

- **corr**: Pearson correlation based ranking. Features having the highest correlation with the target are selected first.
- **NMI** Normalized Mutual Information based ranking. Features having the highest NMI with the target are selected first.
- **RF** The data is first fitted with a Random Forest (300 trees), and features are ranked according to their impurity-based importance.
- **SISSO** The data is first fitted by the SISSO model without applying any operator on the feature set, i.e. only primary features are used (rung set to 0). Each n-th dimension of the final model corresponds to the n-th descriptor. See [8] for further details.
- **OMP** Same strategy as SISSO, but here the SIS-space is restricted to 1. The algorithm thus reduces to an Orthogonal Matching Pursuit (OMP).

Before comparing the different algorithms, it is worth giving some comments about the SISO algorithm used as a feature selection method. Although it is often seen as a dimensionality reduction technique, it can however not be used as such for feature selection in the same generality as the other ones. SISO provides a general framework for selecting the best few descriptors from an immense set of candidates. From our findings, few means no more than 10 descriptors, as it is computationally not feasible to go beyond this value due to the exponential time complexity. This is not an issue for the original aim of SISO (which consists in a low dimensional model), but surely is when used together with a neural network, where the optimal amount is typically some hundreds of features. Therefore, when going beyond the 10th feature, we simplified SISO to OMP, which scales linearly with the number of features.

Figure S9(a) shows the test error on the vibrational entropy at 305 K for the different models (MODNet substituted with different selection algorithms) for the first 10 selected features. The training size is fixed to 1100 samples. There is a clear distinction between redundancy based techniques (MOD and SISO) and non-redundancy based techniques (corr, NMI and RF). Accounting for redundancy is clearly important when using only a few features. In this particular scenario SISO outperforms MOD-selection.

However, in order to construct the best possible model, one should go much further than 10 features. Figure S9(b) depicts the same error but in function of the training size, all other hyper-parameters being optimized. The number of optimal features is often chosen to be around 300 features. SISO is therefore replaced by the OMP. It can be seen how MODNet outperforms all other selection algorithms, particularly at low sample size. The OMP method performs poorly due to wrongly chosen features which result in overfitting.

As an additional experiment, we aim to measure how well a feature selection algorithm is able to capture the important features, when only given a limited amount of labeled samples. We measure this by first running each selection algorithm on the *total dataset*, keeping the best 300 features, which forms the best approximation of optimal features for each algorithm. As a second step, we do the same but on a *sampled subsets* of varying size. The Jaccardian similarity between the 300 features found on the subset and total dataset is represented in Figure S9(c). Note that this metric only represents how fast an algorithm converges in terms of chosen features, but doesn't necessarily mean that the selected features are worthwhile. As can be seen, the similarity increases when the training size increases (with some exceptions due to sampling variance), as the sampled dataset approaches the total dataset. The correlation method shows to provide the highest similarity for all training sizes. This can be explained by the simpler nature of the algorithm: measuring linear dependence require less samples than more complex non-linear dependences. The MOD and NMI approaches show to have a steeper increase in similarity than the RF-approach, while the three are non-linear approaches. Finally, the OMP algorithm has a low Jaccardian similarity, and this for the whole range of subsets. Additional experiments on the OMP showed that the similarity between features chosen on the different sampled subsets are also low, in contrast with the other methods. This clearly shows that a significant variance in selected features is found when slightly changing the training set, which is not desirable. Therefore the OMP method should be avoided. This also explains the poor performance in Figure S9(b).

From these results, one can conclude that depending on the number of features required, some algorithms should be preferred above others. For the first few features, accounting for redundancy seems critical, with SISO performing best, but limited in dimensionality. MOD-selection performs reasonably well in this regime but can provide an unlimited amount of ranked features. In our framework where the number of features is optimized and thus not limited, MOD-selection is found to be the best performing algorithm.

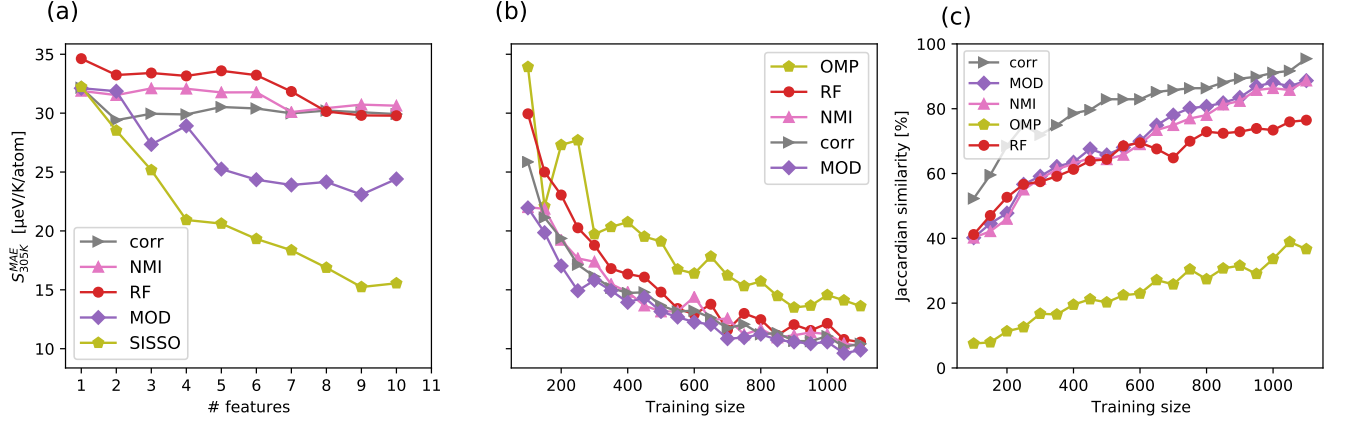

Figure S9. (a) Test error on the vibrational entropy at 305K for different feature selection algorithms, as a function of the first few features for 1100 training samples. (b) Test error on the vibrational entropy at 305K for different feature selection algorithms as a function of the training size with other parameters being optimized over a fixed grid. Models are constructed by replacing the selection algorithm in MODNet by a Pearson correlation (corr), Normalized Mutual Information (NMI), Random Forest (RF), SISSO, and orthogonal matching pursuit (OMP). (c) Jaccardian similarity of the 300 first selected features on a sampled training set of size  $n$ , and the total dataset (1245 samples) as a function of  $n$ , for different feature selection algorithms.

## H. MODNet and vibrational thermodynamic data

### 1. Supplemental results

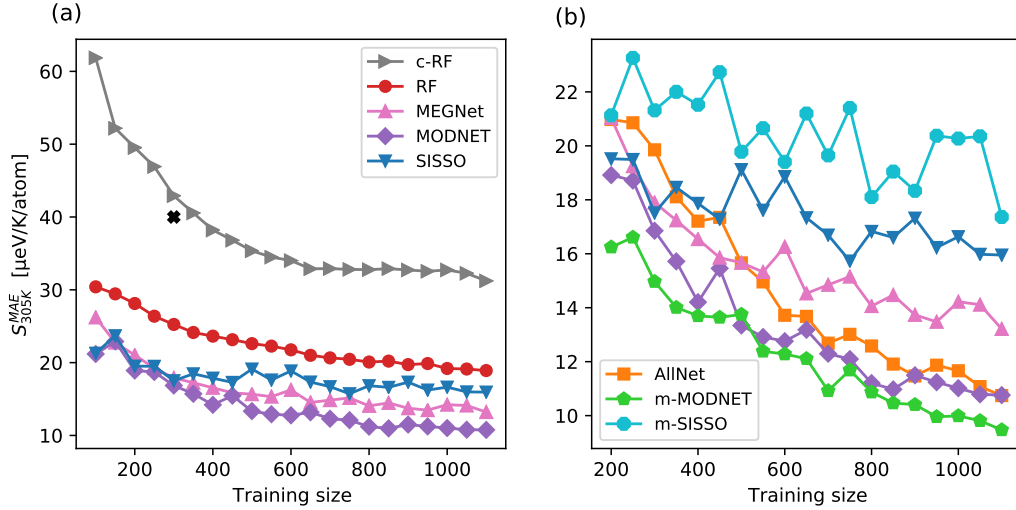

Figure S10. Test MAE on the vibrational entropy at 305K ( $S_{305K}$  in  $\mu\text{eV/K/atom}$ ) as a function of the training size for various strategies (see main text for a detailed description). (a) Random Forest (RF) approaches are compared to neural-network models (Nets) and SISSO. The black cross indicates the RF result of Legrain *et al.* [9] based on 300 materials. (b) Best performing models and multi-target approaches are confronted.

Figure 2 in the main letter contains a quantitative comparison of different ML models on the vibrational entropy at 305K. The error density distribution was given for three training sizes. For sake of completeness, we report here, in Figure S10, the mean absolute error for various training sizes (ranging from 100 to 1100 in steps of 50) for the same ML methods (please refer to the main text for the different approaches). Moreover, the expected error from a

previous work by Legrain *et al.* on vibrational thermodynamics based on a RF on the composition alone trained on 300 materials, is indicated by a black cross on this figure [9].

From Figure S10 (a), it can be seen that neural-network models perform better than RF approaches whatever the size of the dataset. This can probably be explained by the rather complex non-linear nature of the regression problem. Furthermore, MODNet leads to smaller errors than MEGNet confirming our previous finding that it is more appropriate for small datasets. For the RF approaches, adding structural features is clearly beneficial, as explained in the main text. SISSO has a comparable mean error than best methods around and below 300 samples. However beyond this point, no significant improve in mean error is seen, in contrast with other algorithms.

In Fig. S10(b), best performing methods are confronted. Whatever the training size in the range available here, adding feature selection (compare AllNet to MODNet) reduces the prediction error. This is especially true at low sample sizes, where helping the learning algorithm by giving the right descriptors is crucial. The MEGNet model with transfer learning performs somewhat better than AllNet below 500 samples but it is outperformed beyond this point by all neural network models based on physical descriptors. Finally, our joint-learning approach that adds all other thermodynamic properties (m-MODNet) shows in average a slight improve in accuracy ( $\sim 8\%$ ). This is in contrast with m-SISSO, which does not show an improve in accuracy with respect to single target learning.

## 2. Expected generalization error

The m-MODNet was trained on four vibrational properties from 5 to 800 K: entropy, enthalpy, specific heat and Helmholtz free energy. Although the vibrational entropy at 305 K was systematically used to compare against other models, excellent performance was also found on the other properties. Table S5 contains the MAE for these four properties at 25, 305 and 705 K. Typical values of the corresponding properties found in the dataset are also given to compare against the error. As an example, we illustrate the prediction on  $Li_2O$  in Fig. S11, which is a good representation of the typical observed error.

Table S5. MAE of various vibrational properties as predicted from the MODNet.

| Property                  | Typical values        | MODNet MAE ( $\times 10^{-3}$ ) | MODNet MAX MAE ( $\times 10^{-3}$ ) |
|---------------------------|-----------------------|---------------------------------|-------------------------------------|
| $S_{25K}$ [meV/K/atom]    | $\sim 10^{-5}$ - 0.1  | 2.5                             | 2.9                                 |
| $S_{305K}$ [meV/K/atom]   | $\sim 0.03$ - 0.7     | 9.5                             | 11.3                                |
| $S_{705K}$ [meV/K/atom]   | $\sim 0.1$ - 0.9      | 10.8                            | 12.6                                |
| $H_{25K}$ [eV/atom]       | $\sim 7$ - 180        | 2.6                             | 2.9                                 |
| $H_{305K}$ [eV/atom]      | $\sim -130$ - 180     | 6.9                             | 7.5                                 |
| $H_{705K}$ [eV/atom]      | $\sim -460$ - 150     | 8.2                             | 9.7                                 |
| $C_{v,25K}$ [meV/K/atom]  | $\sim 10^{-5}$ - 0.16 | 3.2                             | 3.8                                 |
| $C_{v,305K}$ [meV/K/atom] | $\sim 0.07$ - 0.26    | 2.6                             | 3.0                                 |
| $C_{v,705K}$ [meV/K/atom] | $\sim 0.18$ - 0.26    | 1.6                             | 1.9                                 |
| $U_{25K}$ [eV/atom]       | $\sim 10$ - 180       | 2.2                             | 2.6                                 |
| $U_{305K}$ [eV/atom]      | $\sim 80$ - 200       | 1.6                             | 1.6                                 |
| $U_{705K}$ [eV/atom]      | $\sim 180$ - 270      | 1.2                             | 1.4                                 |

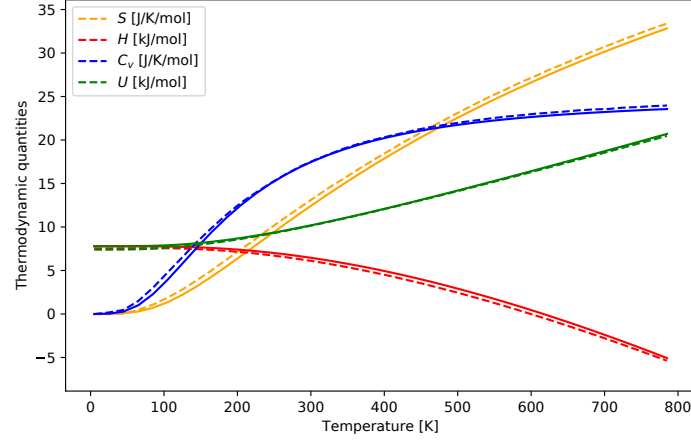

Figure S11. MODNet predictions (dashed line) and DFPT values (solid line) for the thermodynamic quantities of  $\text{Li}_2\text{O}$  (MPID: mp-1960) as a function of the temperature.

- 
- [1] G. Petretto, S. Dwaraknath, H. P. C. Miranda, D. Winston, M. Giantomassi, M. J. van Setten, X. Gonze, K. A. Persson, G. Hautier, and G.-M. Rignanese, *Sci. Data* **5**, 180065 (2018).
  - [2] F. Naccarato, F. Ricci, J. Suntivich, G. Hautier, L. Wirtz, and G.-M. Rignanese, *Phys. Rev. Materials* **3**, 044602 (2019).
  - [3] V. Botu and R. Ramprasad, *Int. J. Quantum Chem.* **115**, 1074 (2015).
  - [4] A. Seko, H. Hayashi, K. Nakayama, A. Takahashi, and I. Tanaka, *Phys. Rev. B* **95**, 144110 (2017).
  - [5] S. Kotochigova, Z. H. Levine, E. L. Shirley, M. D. Stiles, and C. W. Clark, *Phys. Rev. A* **55**, 191 (1997).
  - [6] L. Ward, R. Liu, A. Krishna, V. I. Hegde, A. Agrawal, A. Choudhary, and C. Wolverton, *Phys. Rev. B* **96**, 024104 (2017).
  - [7] J. Heaton, in *SoutheastCon 2016* (IEEE, Norfolk, VA, USA, 2016) pp. 1–6.
  - [8] R. Ouyang, S. Curtarolo, E. Ahmetcik, M. Scheffler, and L. M. Ghiringhelli, *Phys. Rev. Materials* **2**, 083802 (2018).
  - [9] F. Legrain, J. Carrete, A. van Roekeghem, S. Curtarolo, and N. Mingo, *Chem. Mater.* **29**, 6220 (2017).
